# Supplementary material for: Production of non-local quartets and phase-sensitive entanglement in a superconducting beam splitter
Source: arXiv:1102.2355 ancillary file (2011-06-25)
Supplement: Supplementary file 1 [file EPAPS_Freyn_2011.pdf]

# **Production of non-local quartets and phase-sensitive entanglement in a three-terminal Josephson set-up: EPAPS**

Axel Freyn<sup>1</sup>, Benoit Douçot<sup>2</sup>, Denis Feinberg<sup>1</sup>, Régis Mélin<sup>1\*</sup>

<sup>1</sup> *Institut NEEL, CNRS and Université Joseph Fourier,  
BP 166, F-38042 Grenoble Cedex 9, France and*

<sup>2</sup> *Laboratoire de Physique Théorique et des Hautes Energies,  
CNRS UMR 7589, Universités Paris 6 et 7,  
4 Place Jussieu, 75252 Paris Cedex 05*

(Dated: April 28, 2011)

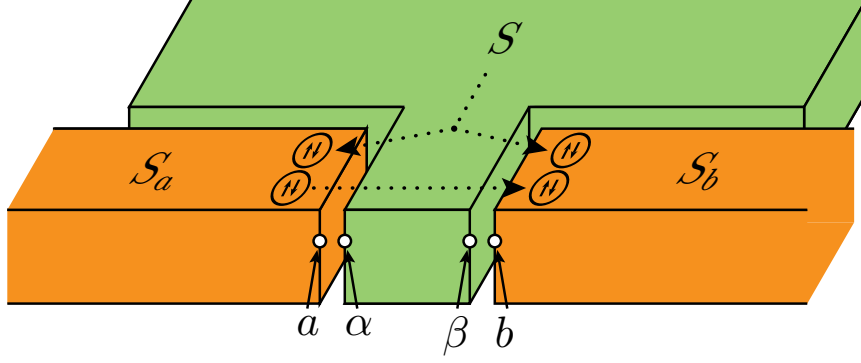

FIG. 1: (Color online). Schematics of a  $S_aISIS_b$  structure and of the dCAR and dEC processes. dCAR trasmits a non-local quartet (with charge  $4e$ ) as two pairs (with charge  $2e$ ) in  $S_a$  and  $S_b$ . dEC transfers a pair from  $S_a$  (with charge  $2e$ ) as a pair in  $S_b$  (with charge  $2e$ ). The superconductor  $S$  has a gap  $\Delta_S$  larger than the gap  $\Delta \equiv \Delta_a, \Delta_b$  in  $S_a$  and  $S_b$ .

## I. DETAILS ON THE MICROSCOPIC CALCULATIONS IN EQUILIBRIUM (FIG. 2 IN THE LETTER)

### A. Hamiltonians

The electrode  $S_a$  (see Fig. 1) is described by a BCS Hamiltonian on a three-dimensional tight-binding lattice:

$$\mathcal{H}_{BCS,a} = -W_a \sum_{\langle \mathbf{x}_a, \mathbf{y}_a \rangle, \sigma} (c_{\mathbf{x}_a, \sigma}^+ c_{\mathbf{y}_a, \sigma} + h.c.) + \Delta \sum_{\mathbf{x}_a} (\exp(i\phi_a) c_{\mathbf{x}_a, \uparrow}^+ c_{\mathbf{x}_a, \downarrow}^+ + h.c.), \quad (1)$$

where  $\sigma$  is the projection of the spin in the direction of a quantization axis. The first summation runs over all pairs  $\langle \mathbf{x}_a, \mathbf{y}_a \rangle$  of neighboring tight-binding sites in  $S_a$ , and  $\mathbf{x}_a$  in the second summation runs over all tight-binding sites in  $S_a$ . The energy  $W_a$  is the hopping amplitude between neighboring tight-binding sites in electrode  $S_a$ , and  $\Delta \exp(i\phi_a)$  is the complex order parameter with amplitude  $\Delta$  and phase  $\phi_a$ . The values of  $\Delta$  and  $\phi_a$  are homogeneous in space in the considered quasi-equilibrium situations (with weak currents in comparison to the critical currents).

Similarly, the Hamiltonians of electrodes  $S_a$  and  $S$  are given by

$$\mathcal{H}_{BCS,b} = -W_b \sum_{\langle \mathbf{x}_b, \mathbf{y}_b \rangle, \sigma} (c_{\mathbf{x}_b, \sigma}^+ c_{\mathbf{y}_b, \sigma} + h.c.) + \Delta \sum_{\mathbf{x}_b} (\exp(i\phi_b) c_{\mathbf{x}_b, \uparrow}^+ c_{\mathbf{x}_b, \downarrow}^+ + h.c.) \quad (2)$$

$$\mathcal{H}_{BCS,S} = -W_S \sum_{\langle \mathbf{x}_S, \mathbf{y}_S \rangle, \sigma} (c_{\mathbf{x}_S, \sigma}^+ c_{\mathbf{y}_S, \sigma} + h.c.) + \Delta_S \sum_{\mathbf{x}_S} (\exp(i\phi_S) c_{\mathbf{x}_S, \uparrow}^+ c_{\mathbf{x}_S, \downarrow}^+ + h.c.). \quad (3)$$

The different physical quantities are expressed with the combinations  $\delta\phi_a = \phi_a - \phi_S$  and  $\delta\phi_b = \phi_b - \phi_S$ .

The part of the Hamiltonian coupling the different electrodes is given by

$$\mathcal{H}_{a-S} = -t_{a,S} \sum_{\langle \mathbf{x}_a, \mathbf{y}_S \rangle, \sigma} (c_{\mathbf{x}_a, \sigma}^+ c_{\mathbf{y}_S, \sigma} + h.c.) \quad (4)$$

$$\mathcal{H}_{b-S} = -t_{b,S} \sum_{\langle \mathbf{x}_b, \mathbf{y}_S \rangle, \sigma} (c_{\mathbf{x}_b, \sigma}^+ c_{\mathbf{y}_S, \sigma} + h.c.), \quad (5)$$

where the real-valued  $t_{a,S}$  and  $t_{b,S}$  are the hopping amplitudes between  $S_a$  and  $S$ , and between  $S_b$  and  $S$ . The summations in Eq. (4) and (5) run over the pairs of tight-binding sites at the interface. For instance,  $\mathbf{x}_a$  runs over the  $S_a$  side of the interface, and  $\mathbf{y}_S$  is its counterpart in the  $S$  side of the interface.

If  $W \equiv W_a = W_b = W_S$  and  $t_0 \equiv t_{a,S} = t_{b,S}$ , the dimensionless normal state transmission coefficient of each contact is given by

$$T_N = \frac{4(t_0/W)^2}{(1 + (t_0/W)^2)^2}. \quad (6)$$

The normal state transmission coefficient is given by  $T_N \simeq 4(t_0/W)^2$  in the tunnel limit  $t_0 \ll W$ , and it is given by  $T_N = 1$  for highly transparent contacts with  $t_0 = W$ .

## B. Nambu Green's functions in equilibrium

Keldysh perturbation theory for the Hamiltonian given by Eqs. (1)-(5) is summed to infinite orders in the spirit of Refs. 1–3, making it possible to treat interfaces with arbitrary transparency, in the case where no bias voltages are applied.

The “local” advanced Nambu Green's functions at energy  $\omega$  for the superconducting electrodes isolated from each other are given by:

$$\hat{g}_{a,a}^A(\omega) = \frac{1}{W_a \sqrt{(\Delta_a)^2 - (\omega - i\eta)^2}} \begin{pmatrix} -(\omega - i\eta) & \Delta_a \exp(i\phi_a) \\ \Delta_a \exp(-i\phi_a) & -(\omega - i\eta) \end{pmatrix} \quad (7)$$

$$\hat{g}_{b,b}^A(\omega) = \frac{1}{W_b \sqrt{(\Delta_b)^2 - (\omega - i\eta)^2}} \begin{pmatrix} -(\omega - i\eta) & \Delta_b \exp(i\phi_b) \\ \Delta_b \exp(-i\phi_b) & -(\omega - i\eta) \end{pmatrix} \quad (8)$$

$$\hat{g}_{\alpha,\alpha}^A(\omega) = \hat{g}_{\beta,\beta}(\omega) = \frac{1}{W_S \sqrt{(\Delta_S)^2 - (\omega - i\eta)^2}} \begin{pmatrix} -(\omega - i\eta) & \Delta_S \exp(i\phi_S) \\ \Delta_S \exp(-i\phi_S) & -(\omega - i\eta) \end{pmatrix}. \quad (9)$$

The “non-local” Green’s functions coupling the two interfaces are given by

$$\begin{aligned} \hat{g}_{\alpha,\beta}^A(\omega) = \hat{g}_{\beta,\alpha}^A(\omega) = \frac{1}{W_S} \exp\left(-\frac{R_{\alpha,\beta}}{\xi(\omega - i\eta)}\right) \times \\ \left\{ \frac{1}{\sqrt{(\Delta_S)^2 - (\omega - i\eta)^2}} \begin{pmatrix} -(\omega - i\eta) & \Delta_S \exp(i\phi_S) \\ \Delta_S \exp(-i\phi_S) & -(\omega - i\eta) \end{pmatrix} \cos(k_{F,S} R_{\alpha,\beta}) \right. \\ \left. + \begin{pmatrix} 1 & 0 \\ 0 & -1 \end{pmatrix} \sin(k_{F,S} R_{\alpha,\beta}) \right\}, \end{aligned} \quad (10)$$

where  $k_{F,S}$  is the Fermi wave-vector in S, and  $R_{\alpha,\beta}$  is the distance separating the tight-binding sites  $\alpha$  and  $\beta$  at the S side of the interfaces  $S_a\text{IS}$  and  $\text{SIS}_b$  (see Fig. 1). The notation  $\xi(\omega - i\eta)$  is the coherence length at energy  $\omega - i\eta$ , where  $\eta$  is a small positive line-width broadening.

### C. Dyson equations in equilibrium

The Dyson equations take generically the form  $\hat{G} = \hat{g} + \hat{g} \otimes \hat{\Sigma} \otimes \hat{G}$ , where  $\otimes$  is a summation over the spatial labels of the self-energy, and a convolution over the time arguments. In the absence of applied voltage as it is the case for Fig. 2, the latter is Fourier transformed as a product of Green’s functions evaluated at frequency  $\omega$ . For instance, the Dyson equations take the form

$$\hat{G}_{\alpha,\alpha}(\omega) = \hat{g}_{\alpha,\alpha}(\omega) + \hat{g}_{\alpha,\alpha}(\omega) \hat{\Sigma}_{\alpha,a} \hat{G}_{a,\alpha}(\omega) + \hat{g}_{\alpha,\beta}(\omega) \hat{\Sigma}_{\beta,b} \hat{G}_{b,\alpha}(\omega) \quad (11)$$

$$\hat{G}_{\beta,\alpha}(\omega) = \hat{g}_{\beta,\alpha}(\omega) + \hat{g}_{\alpha,\alpha}(\omega) \hat{\Sigma}_{\alpha,a} \hat{G}_{a,\alpha}(\omega) + \hat{g}_{\beta,\beta}(\omega) \hat{\Sigma}_{\beta,b} \hat{G}_{b,\alpha}(\omega), \quad (12)$$

where the Green’s functions  $\hat{g}_{k,l}(\omega)$  are the “bare” ones for the uncoupled electrodes, and  $\hat{G}_{k,l}(\omega)$  denotes the fully dressed ones, containing all possible multiple scattering processes within one interface, or between the two interfaces. The Nambu self-energy  $\hat{\Sigma}_{k,l}$  corresponds to interfacial scattering:

$$\hat{\Sigma}_{a,\alpha} = \hat{\Sigma}_{\alpha,a} = t_{a,S} \begin{pmatrix} 1 & 0 \\ 0 & -1 \end{pmatrix} \quad (13)$$

$$\hat{\Sigma}_{b,\beta} = \hat{\Sigma}_{\beta,b} = t_{b,S} \begin{pmatrix} 1 & 0 \\ 0 & -1 \end{pmatrix}. \quad (14)$$

Starting from Eqs. (11) and (12) and using again the Dyson equation leads to the following closed set of equations for  $\hat{G}_{\alpha,\alpha}(\omega)$  and  $\hat{G}_{\beta,\alpha}(\omega)$ :

$$\left(\hat{I} - \hat{K}_{\alpha,\alpha}(\omega)\right) \hat{G}_{\alpha,\alpha}(\omega) - \hat{K}_{\alpha,\beta}(\omega) \hat{G}_{\beta,\alpha}(\omega) = \hat{g}_{\alpha,\alpha}(\omega) \quad (15)$$

$$-\hat{K}_{\beta,\alpha}(\omega) \hat{G}_{\alpha,\alpha}(\omega) + \left(\hat{I} - \hat{K}_{\beta,\beta}(\omega)\right) \hat{G}_{\beta,\alpha}(\omega) = \hat{g}_{\beta,\alpha}(\omega), \quad (16)$$

where the expression of the  $\hat{K}_{k,l}(\omega)$  involves only the set of the  $\hat{g}_{k,l}(\omega)$ . Using Eq. (16) to express  $\hat{G}_{\beta,\alpha}(\omega)$  as a function of  $\hat{G}_{\alpha,\alpha}(\omega)$  and injecting this expression in Eq. (15) leads to a closed expression for  $\hat{G}_{\alpha,\alpha}(\omega)$  which involves the inversion of only  $2 \times 2$  matrices. The value of all Green's functions is obtained by using again the Dyson equations. The perturbative expansion of Ref. 4 can be carried out if propagation in S is damped by a gap  $\Delta_S$  large compared to  $\Delta \equiv \Delta_a = \Delta_b$ ,

#### D. Expression of the current and cross-correlations in equilibrium

The current operator through the link a- $\alpha$  (see Fig. 1) is given by

$$\hat{I}_{a,\alpha}(t) = t_{a,S} \sum_{\sigma} \left( c_{\alpha,\sigma}^+(t) c_{a,\sigma}(t) - c_{a,\sigma}^+(t) c_{\alpha,\sigma}(t) \right). \quad (17)$$

The average current is the expectation value of Eq. (17). The current-current cross-correlations are given by

$$S_{a,b}(t, t') = \langle \delta \hat{I}_a(t + t') \hat{I}_b(t) \rangle + \langle \delta \hat{I}_b(t) \delta \hat{I}_a(t + t') \rangle, \quad (18)$$

where  $\langle \dots \rangle$  denotes the average value.

The spectral average current  $I_{a,\alpha}(\omega)$  and the spectral cross-correlations  $S_{a,b}(\omega)$  are related as follows to the Keldysh Green's function<sup>1-3</sup>:

$$I_{a,\alpha}(\omega) = \frac{2e}{h} \left[ \hat{\Sigma}_{a,\alpha} \hat{G}_{\alpha,a}^{+,-}(\omega) - \hat{\Sigma}_{\alpha,a} \hat{G}_{a,\alpha}^{+,-}(\omega) \right]_{1,1} \quad (19)$$

$$S_{a,b}(\omega) = \frac{2e^2}{h} t_a t_b \text{Tr} \left[ \hat{G}_{b,a}^{+,-}(\omega) \hat{G}_{\alpha,\beta}^{-,+}(\omega) + \hat{G}_{\beta,\alpha}^{+,-}(\omega) \hat{G}_{a,b}^{-,+}(\omega) \right. \\ \left. - \hat{G}_{b,\alpha}^{+,-}(\omega) \hat{G}_{a,\beta}^{-,+}(\omega) - \hat{G}_{\beta,a}^{+,-}(\omega) \hat{G}_{a,b}^{-,+}(\omega) \right], \quad (20)$$

where the trace is a summation over the Nambu labels. The Keldysh Green's functions  $\hat{G}^{+,-}(\omega)$  and  $\hat{G}^{-,+}(\omega)$  are given in Ref. 1-3. Finally, a summation over all pairs of sites (a,b) at the interfaces  $S_a$  IS a  $SIS_b$  is carried out.

### E. Details on the non-local inductance and cross-correlations in the specific case of the tunnel limit (Fig. 2a in the Letter)

Both dCAR and dEC contribute to the supercurrent at zero temperature in the tunnel limit. Their contributions has the following phase dependence:  $\sin(\delta\phi_a + \delta\phi_b)$  for dCAR and to  $\sin(\delta\phi_a - \delta\phi_b)$  for dEC. The transmission mode dCAR is

$$\langle\langle g_{\alpha,\beta,1,2}(\omega)g_{\beta,\alpha,1,2}(\omega)\rangle\rangle = \frac{1}{2(W_S)^2} \frac{(\Delta_S)^2}{(\Delta_S)^2 - (\omega - i\eta)^2} \exp\left(-\frac{2R_{\alpha,\beta}}{\xi(\omega - i\eta)}\right), \quad (21)$$

where  $\phi_S = 0$  was supposed without loss of generality. The notation  $\langle\langle \dots \rangle\rangle$  is used for averaging over the Fermi oscillations:

$$\langle\langle f(R, \omega) \rangle\rangle = \frac{k_F}{2\pi} \int_{R-\pi/k_F}^{R+\pi/k_F} f(r, \omega) dr. \quad (22)$$

The transmission mode dEC has a non-trivial change of sign from negative to positive as  $\omega$  increases above  $\omega = \Delta_S/\sqrt{2}$ :

$$\langle\langle g_{\alpha,\beta,1,1}(\omega)g_{\beta,\alpha,2,2}(\omega)\rangle\rangle = \frac{1}{2(W_S)^2} \frac{2(\omega - i\eta)^2 - (\Delta_S)^2}{(\Delta_S)^2 - (\omega - i\eta)^2} \exp\left(-\frac{2R_{\alpha,\beta}}{\xi(\omega - i\eta)}\right). \quad (23)$$

The bound states are close to the gap in the tunnel limit and the current  $I_a$  has the following phase dependence:  $\sin(\delta\phi_a + \delta\phi_b) + \sin(\delta\phi_a - \delta\phi_b)$ . The quantity  $-L_{a,b} = -\partial I_a / \partial \phi_b$  has the phase dependence  $2\sin(\delta\phi_a)\sin(\delta\phi_b)$ , which matches Fig. 2a in the Letter.

## II. DETAILS ON FINITE BIAS VOLTAGES

Perturbative expansions in the tunnel amplitude are carried out for the current, and for the current-current cross-correlations in the presence of finite applied voltages. Only the lowest order contribution for small values of interface transparency (tunnel limit) is retained. The contribution of all transmission modes is evaluated, including dCAR and dEC.

The appearance of a dc Josephson current for non-local quartets in a three-terminal  $S_a\text{ISIS}_b$  structure does not rely on whether the interface transparency is small or large. The energy required for correlated transmission of two pairs from S into  $S_a$  and  $S_b$  is  $2e(V_a + V_b - 2V_S)$ , which vanishes if  $V_a + V_b - 2V_S = 0$ , resulting in a time-independent dc-Josephson current for non-local quartets, whatever the values of the interface transparencies. Similarly, the energy for transmitting a pair from  $S_a$  to  $S_b$  by dEC is  $2e(V_b - V_a)$  for all  $V_S$ , and it vanishes if  $V_a = V_b$ .

The can be seen as follows from the Fourier transform of the current. We note  $\omega_a = eV_a$  and  $\omega_b = eV_b$ . The phase differences are given by  $\delta\phi_a(t) = \omega_a t + \delta\phi_a$  and  $\delta\phi_b(t) = \omega_b t + \delta\phi_b$ . The Fourier expansion for the average current  $I_a(t)$  is given by<sup>2</sup>

$$I_a(t) = \int d\omega \sum_{n_a, n_b} \exp(in_a \omega_a t) \exp(-in_b \omega_b t) I_{a, n_a, n_b}(\omega). \quad (24)$$

Assuming  $V_a = -V_b$  and thus  $\omega_a + \omega_b = 0$ , the dc-components of  $I_a$  are given by:

$$I_{a, dc} = \int d\omega \sum_{n_a, n_b} \delta_{n_a + n_b, 0} I_{a, n_a, n_b}(\omega). \quad (25)$$

The first terms  $\int d\omega [I_{a, 1, -1}(\omega) + I_{a, -1, 1}(\omega)]$  lead to the dc-component of the supercurrent induced by opposite voltages on  $S_a$  and  $S_b$ , corresponding to AR, CAR, EC, dCAR and dEC (see Fig. 1 in the Letter).

There is a parallel between CAR, EC and dCAR, dEC: in perturbation theory, transmitting a *single* electron (charge  $e$ ) at a tunnel junction appears at order  $T_N$ . Splitting pairs from S as two quasi-particles in the *double* junction  $N_a \text{ISIN}_b$  by CAR is of order  $(T_N)^2$ . Transmission of a Josephson current of pairs at a *single* SIS junction is of order  $T_N$ . Splitting a supercurrent in  $S_a \text{ISIS}_b$  by dCAR with *two* Josephson junctions spatially separated by  $\xi_S(0)$  is also of order  $(T_N)^2$ . Our formalism allows to treat also arbitrary values of interface transparency.

### III. DETAILS ON ENTANGLEMENT

#### A. Entanglement in superconducting hybrid structures

The state of a  $S_a \text{IS}_b$  junction with phases  $\phi_a$  and  $\phi_b$  is described by the wave-function

$$|\psi\rangle_{a,b} = \sum_n \exp[in(\phi_a - \phi_b)] |N_a - n\rangle \otimes |N_b + n\rangle, \quad (26)$$

where  $|n \otimes |m\rangle$  refers to  $n$  pairs in  $S_a$ , and  $m$  pairs in  $S_b$ . This state is not entangled if  $N_a$  and  $N_b$  can take arbitrary values, and it is entangled if the total number of pairs  $N_a + N_b$  is fixed.

For a  $S_a \text{ISIS}_b$  double junction, the ground state is given by the product

$$|\psi\rangle = |\psi\rangle_{a,S} |\psi\rangle_{S,b} \quad (27)$$

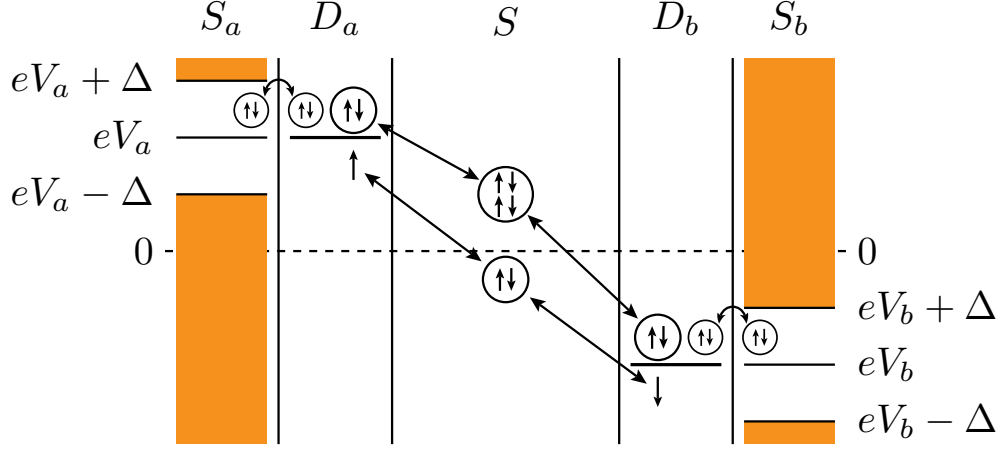

FIG. 2: Schematics of the  $S_a D_a S D_b S_b$  junction in the absence of Coulomb interaction. A spin-degenerate level of  $D_a$  ( $D_b$ ) is resonant with the Fermi level of  $S_a$  ( $S_b$ ) at energy  $eV_a$  ( $eV_b$ ). No level is present at energy  $-eV_a$  ( $-eV_b$ ) in  $D_a$  ( $D_b$ ). The AR, CAR and dCAR processes are shown schematically.

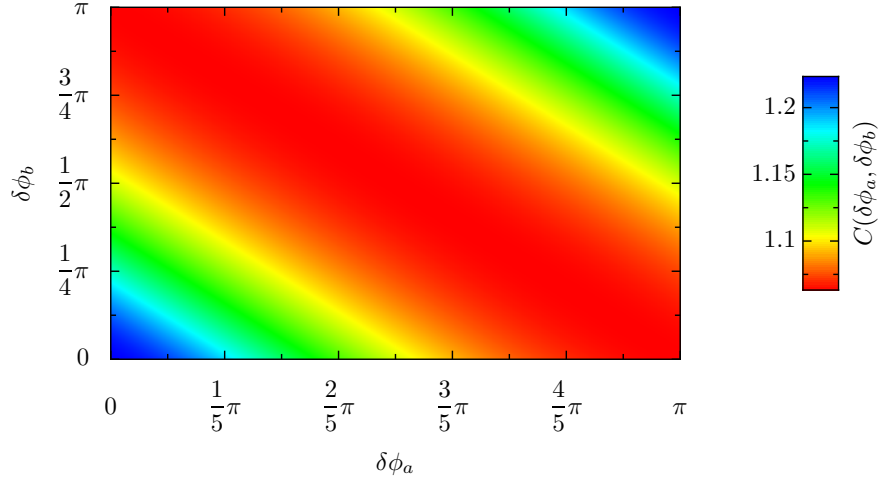

FIG. 3: Variations of the concurrence in the ground state [see Eq. (29)] in the  $(\delta\phi_a, \delta\phi_b)$  plane. The parameters are  $\alpha = 0.2$ ,  $\beta = 0.3$ ,  $\gamma = 0.1$ ,  $U = 0$ . The same qualitative behavior is found for the concurrence of the non-degenerate ground state of the multiplet with a finite value of the Coulomb repulsion  $U$ .

if the distance between the two interfaces is large compared to the coherence length of  $S$ .

In the other limit where the separation between the interfaces is comparable to the



coherence length, the ground state is given by

$$|\psi\rangle = \sum_n \exp[in(\phi_a + \phi_b - 2\phi_S)] |N_a - n\rangle \otimes |N_S + 2n\rangle \otimes |N_b - n\rangle. \quad (28)$$

Eq. (28) is not entangled if a summation over  $N_a$ ,  $N_b$ ,  $N_S$  is carried out, and it is entangled and similar to the state of two coupled Qu-bits if the normal electrodes are replaced by discrete quantum dot energy levels with  $n = 0, 1$ .

### B. Phase-sensitive entanglement for quantum dots in the tunnel limit

Phase-sensitive entanglement between the levels  $D_a$  and  $D_b$  at the Fermi energies of  $S_a$  and  $S_b$  (see Fig. 2) is evaluated via a calculation of the concurrence (see for instance Ref. 5). The concurrence of the ground state at zero temperature is given by

$$C(|\psi\rangle) = \sqrt{2(1 - \text{Tr}(\rho_a^2))}, \quad (29)$$

where  $\rho_a$  is the reduced density matrix obtained after tracing over the subsystem  $b$ . Fig. 3 shows the concurrence in the  $(\delta\phi_a, \delta\phi_b)$  plane, obtained numerically from exact diagonalizations. The concurrence depends on  $\delta\phi_a$  and  $\delta\phi_b$  through the dCAR combination  $\delta\phi_a + \delta\phi_b$ . The concurrence is maximal for  $\delta\phi_a \simeq \delta\phi_b \simeq 0$ , and minimal for  $\delta\phi_a \simeq \delta\phi_b \simeq \pi/2$ . The variations of the cross-correlations with CAR and dCAR in the  $S_a n_a S p_b S_b$  tunnel structure follow closely the variations of the concurrence on Fig. 3, which is qualitatively compatible with the Bell-like argument.

#### IV. COMPARISON BETWEEN THE DIFFERENT SET-UPS

|                                                 |                                              |                                              |                                                                                |
|-------------------------------------------------|----------------------------------------------|----------------------------------------------|--------------------------------------------------------------------------------|
|                                                 | $L_{a,b}(\delta\phi_a, \delta\phi_b) \neq 0$ | $S_{a,b}(\delta\phi_a, \delta\phi_b) \neq 0$ | Demonstration of<br>phase-sensitive<br>entanglement                            |
| $S_a N_a S N_b S_b$<br>(short $N_a$ and $N_b$ ) | $T \geq 0$                                   | $T > 0$ ,<br>thermally activated             | Not directly addressed<br>in the Letter                                        |
| $S_a n S p S_b$                                 | $T \geq 0$                                   | $T > 0$ ,<br>thermally activated             | $T > 0$ , Bell-like argument                                                   |
| $S_a D_a S D_b S_b$                             | $T \geq 0$                                   | $T \geq 0$                                   | $T \geq 0$<br>– concurrence ( $T = 0$ )<br>– Bell-like argument ( $T \geq 0$ ) |

---

\* Electronic address: [Regis.Melin@grenoble.cnrs.fr](mailto:Regis.Melin@grenoble.cnrs.fr)

<sup>1</sup> C. Caroli, R. Combescot, P. Nozières and D. Saint-James, J. Phys. C: Solid St. Phys. **4**, 916 (1971); *ibid.* **5**, 21 (1972).

<sup>2</sup> J.C. Cuevas, A. Martín-Rodero and A. Levy Yeyati, Phys. Rev. B **54**, 7366 (1996)

<sup>3</sup> J.C. Cuevas, A. Martín-Rodero, and A. Levy Yeyati, Phys. Rev. Lett. **82**, 4086 (1999).

<sup>4</sup> R. Mélin and D. Feinberg, Phys. Rev. B **70**, 174509 (2004).

<sup>5</sup> W.K. Wootters, Phys. Rev. Lett. **80**, 2245 (1998).
